# Supplementary material for: Cooperative squeezing of internal and collective spins in an atomic ensemble
Source: arXiv:2503.05446 ancillary file (2025-11-15)
Supplement: Supplementary file 1 [file SI.pdf]

# Supplemental material for "Cooperative squeezing of internal and collective spins in an atomic ensemble"

Youwei Zhang,[1] Shenchao Jin,[2,3] Junlei Duan,[1] Klaus Mølmer,[4]
Guiying Zhang,[5,*] Mingfeng Wang,[6,†] and Yanhong Xiao[1,7,8,‡]

[1]*Department of Physics, State Key Laboratory of Surface Physics and Key Laboratory of Micro and Nano Photonic Structures (Ministry of Education), Fudan University, Shanghai 200433, China*
[2]*CAS Key Laboratory of Quantum Optics and Aerospace Laser Technology and Systems Department, Shanghai Institute of Optics and Fine Mechanics, Chinese Academy of Sciences, Shanghai 201800, China*
[3]*University of Chinese Academy of Sciences, Beijing 100049, China*
[4]*Niels Bohr Institute, University of Copenhagen, Blegdamsvej 17, DK 2100 Copenhagen, Denmark*
[5]*College of Science, Zhejiang University of Technology, Hangzhou 310023, China*
[6]*Department of Physics, Wenzhou University, Zhejiang 325035, China*
[7]*State Key Laboratory of Quantum Optics Technologies and Devices, Institute of Laser Spectroscopy, Shanxi University, Taiyuan, Shanxi 030006, China*
[8]*Collaborative Innovation Center of Extreme Optics, Shanxi University, Taiyuan, Shanxi 030006, China*

## 1. THEORETICAL MODEL

### 1.1 Multilevel Holstein-Primakoff approximation

Our experiment utilizes an ensemble of hot $^{87}$Rb atoms contained in a glass vapor cell. The relevant internal state of each atom is the $F = 2$ manifold of the $5^2S_{1/2}$ ground state, which comprises five Zeeman substates $\{|\psi_\alpha^{(i)}\rangle = |F = 2, m_F = \alpha - 2\rangle_i\}_{\alpha=0}^{4}$. Each atom is initially prepared in the same internal state $|\psi_0^{(i)}\rangle$ via optical pumping, creating the CSS of the atomic ensemble $|\mathrm{CSS}\rangle = |\psi_0\rangle^{\otimes N}$. We take the $x$ axis as the quantization axis, so $|\psi_0^{(i)}\rangle$ is an eigenstate of $\hat{F}_x^{(i)}$, satisfying $\hat{F}_x^{(i)}|\psi_0^{(i)}\rangle = -2|\psi_0^{(i)}\rangle$, while $\hat{F}_y^{(i)}|\psi_0^{(i)}\rangle = \frac{1}{2}(\hat{F}_+^{(i)} + \hat{F}_-^{(i)})|\psi_0^{(i)}\rangle = |\psi_1^{(i)}\rangle$, $\hat{F}_z^{(i)}|\psi_0^{(i)}\rangle = \frac{1}{2i}(\hat{F}_+^{(i)} - \hat{F}_-^{(i)})|\psi_0^{(i)}\rangle = -i|\psi_1^{(i)}\rangle$, where $\hat{F}_\pm^{(i)}$ denote the ladder operators. In this study, we aim for squeezing of the collective spin $\hat{J}_z = \sum_{i=1}^{N}\hat{F}_z^{(i)}$ of the atomic ensemble. The variance of this collective spin component can be calculated to give

$$\left(\Delta\hat{J}_z\right)^2 = \sum_i\left(\Delta\hat{F}_z^{(i)}\right)^2 + 2\sum_{i\neq j}\mathrm{Cov}\left(\hat{F}_z^{(i)}, \hat{F}_z^{(j)}\right). \tag{E1}$$

The first term stands for the total variance of single spins, while the second term represents the correlations (entanglement) between atoms, where $\mathrm{Cov}(\hat{F}_z^{(i)}, \hat{F}_z^{(j)}) = \frac{1}{2}\langle[\hat{F}_z^{(i)}, \hat{F}_z^{(j)}]_+\rangle - \langle\hat{F}_z^{(i)}\rangle\langle\hat{F}_z^{(j)}\rangle$ denotes the covariance between spin observables $\hat{F}_z^{(i)}$ and $\hat{F}_z^{(j)}$ of different atoms, and $[...]_+$ represents the anti-commutator. Our goal is to reduce (squeeze) the variance of $\hat{J}_z$ as much as possible. Clearly, there are two ways to achieve this objective: (i) reducing the variance of $\hat{F}_z^{(i)}$, which can be realized by internal squeezing, and (ii) making the covariance negative, which can be achieved by collective squeezing. Here, we aim to combine these two approaches constructively to minimize the variance of $\hat{J}_z$.

Our atomic system consists of a large number of atoms ($N \sim 10^{11}$). Therefore, it is necessary to employ the Holstein-Primakoff approximation (HPA) [S1] to describe the collective squeezing. For the CSS described above, one can assign to $\hat{J}_y$ and $\hat{J}_z$ a *single* oscillator quadrature variable [S2]

$$\hat{X}_1 = \frac{\hat{J}_y}{\sqrt{2\left(\Delta\hat{J}_y\right)^2_{|\mathrm{CSS}\rangle}}}, \hat{P}_1 = \frac{\hat{J}_z}{\sqrt{2\left(\Delta\hat{J}_z\right)^2_{|\mathrm{CSS}\rangle}}}, \tag{E2}$$

where $(\Delta\hat{O})^2_{|\mathrm{ref}\rangle}$ denotes the variance of $\hat{O}$ associated with the *reference state* $|\mathrm{ref}\rangle = |\mathrm{CSS}\rangle$. Here $(\Delta\hat{J}_y)^2_{|\mathrm{CSS}\rangle} = (\Delta\hat{J}_z)^2_{|\mathrm{CSS}\rangle} = J_x/2$ with macroscopic spin $J_x = NF$, yielding the conventional HPA [S1]: $\hat{X}_1 = \hat{J}_y/\sqrt{J_x}, \hat{P}_1 = \hat{J}_z/\sqrt{J_x}$. The physical meaning of the defined oscillator variables is clear: the reference state $|\mathrm{CSS}\rangle$ corresponds to the vacuum state of a collective mode with annihilation operator $\hat{a}_1 = (\hat{X}_1 - i\hat{P}_1)/\sqrt{2} = \sum_{i=1}^{N}\hat{F}_-^{(i)}/\sqrt{J_x}$, and the first excited state is obtained by applying the creation operator to the reference state $\hat{a}_1^\dagger|\mathrm{CSS}\rangle = \frac{1}{\sqrt{J_x}}\sum_{i=1}^{N}\hat{F}_+^{(i)}|\psi_0\rangle^{\otimes N} = \frac{1}{\sqrt{J_x}}\sum_{i=1}^{N}|\psi_1^{(i)}\rangle|\psi_0\rangle^{\otimes N}_{\neq i} \equiv |1\rangle$—a symmetric collective state where one atom has made the transition $|\psi_0^{(i)}\rangle \mapsto |\psi_1^{(i)}\rangle$. More generally, the symmetric state where $n$ atoms are excited from $|\psi_0^{(i)}\rangle$ to $|\psi_1^{(i)}\rangle$, can be written $|n\rangle = \hat{a}_1^{\dagger n}/\sqrt{n!}\,|0\rangle \propto \sum_{\mathrm{perm}}|\psi_1\rangle^{\otimes n}|\psi_0\rangle^{\otimes(N-n)}$.

In analogy with squeezed state of light [S3], collective spin squeezed states are superpositions of states with even numbers of excitations. A straightforward way to obtain internal squeezing, is the one-axis or two-axis twisting (OAT- or TAT) protocols [S4], which evolve the CSS into a new reference state $|\mathrm{ref}\rangle = |\widetilde{\psi}_0\rangle^{\otimes N}$, where the internally squeezed sate $|\widetilde{\psi}_0^{(i)}\rangle = \hat{U}_0^{(i)}|\psi_0^{(i)}\rangle$. The change of reference state alters the oscillators assigned to $\hat{J}_y$ and $\hat{J}_z$ [S2, S5].

*A pedagocial example of the multi-mode Holstein-Primakoff approximation*

As an example, we take a special orthonormal single-particle basis $\{|\widetilde{\psi}_\alpha^{(i)}\rangle\}_{\alpha=0}^4$ where

$$|\widetilde{\psi}_0^{(i)}\rangle = \frac{1}{\sqrt{2}}\left(|\psi_0^{(i)}\rangle + |\psi_4^{(i)}\rangle\right), \tag{E3a}$$

$$|\widetilde{\psi}_1^{(i)}\rangle = \frac{1}{\sqrt{2}}\left(|\psi_0^{(i)}\rangle - |\psi_4^{(i)}\rangle\right), \tag{E3b}$$

$$|\widetilde{\psi}_2^{(i)}\rangle = |\psi_2^{(i)}\rangle, \tag{E3c}$$

$$|\widetilde{\psi}_3^{(i)}\rangle = \frac{1}{\sqrt{2}}\left(|\psi_1^{(i)}\rangle + |\psi_3^{(i)}\rangle\right), \tag{E3d}$$

$$|\widetilde{\psi}_4^{(i)}\rangle = \frac{1}{\sqrt{2}}\left(|\psi_1^{(i)}\rangle - |\psi_3^{(i)}\rangle\right). \tag{E3e}$$

Corresponding to these basis, we find $\hat{F}_y^{(i)}|\widetilde{\psi}_0^{(i)}\rangle = |\widetilde{\psi}_3^{(i)}\rangle$ and $\hat{F}_z^{(i)}|\widetilde{\psi}_0^{(i)}\rangle = -i|\widetilde{\psi}_4^{(i)}\rangle$, which are different from the case of the CSS basis, where both $\hat{F}_y^{(i)}$ and $\hat{F}_z^{(i)}$ introduce the same state transition, namely $|\psi_0^{(i)}\rangle \to |\psi_1^{(i)}\rangle$. As a result, the collective operators $\hat{J}_{y,z}$ will be assigned to two different oscillators

$$\hat{X}_3 = \frac{\hat{J}_y}{\sqrt{2\left(\Delta\hat{J}_y\right)^2_{|\mathrm{ref}\rangle}}}, \hat{P}_4 = \frac{\hat{J}_z}{\sqrt{2\left(\Delta\hat{J}_z\right)^2_{|\mathrm{ref}\rangle}}}. \tag{E4}$$

The two collective spin components, $\hat{J}_y$ and $\hat{J}_z$, are associated with two separate oscillator degrees of freedom, as we see that $[\hat{X}_3, \hat{P}_4] \propto [\hat{J}_y, \hat{J}_z] \propto \hat{J}_x \approx 0$ in the reference state of Eq. (E3a).

For an arbitrary orthonormal single-particle basis $\{|\widetilde{\psi}_\alpha^{(i)}\rangle\}_{\alpha=0}^4$, four atomic oscillators are required for describing the collective spin components $\hat{J}_{y,z}$ [S2]. To expand $\hat{J}_{y,z}$ in atomic oscillators for a general basis $\{|\widetilde{\psi}_\alpha^{(i)}\rangle\}_{\alpha=0}^4$, we use the completeness relation $\sum_{\alpha=0}^4 |\widetilde{\psi}_\alpha^{(i)}\rangle\langle\widetilde{\psi}_\alpha^{(i)}| = 1$ and write:

$$\hat{J}_y \equiv \sum_{i=1}^N \hat{F}_y^{(i)} = \sum_{\alpha,\beta} J_{\alpha\beta}^y \hat{\Sigma}_{\alpha\beta}, \tag{E5}$$

$$\hat{J}_z \equiv \sum_{i=1}^N \hat{F}_z^{(i)} = \sum_{\alpha,\beta} J_{\alpha\beta}^z \hat{\Sigma}_{\alpha\beta}, \tag{E6}$$

where we have defined the collective spin operators $\hat{\Sigma}_{\alpha\beta} = \sum_{i=1}^N |\widetilde{\psi}_\alpha^{(i)}\rangle\langle\widetilde{\psi}_\beta^{(i)}|$ and the expansion coefficients $J_{\alpha\beta}^{y,z} = \langle\widetilde{\psi}_\alpha^{(i)}|\hat{F}_{y,z}^{(i)}|\widetilde{\psi}_\beta^{(i)}\rangle$. The collective operator $\hat{\Sigma}_{\alpha\beta}$ can induce the atomic transition $|\widetilde{\psi}_\beta^{(i)}\rangle \to |\widetilde{\psi}_\alpha^{(i)}\rangle$ of a single atom. We here mainly focus on the case that the collective control does not drive the atomic system far away from the reference state. In this case, we have $\hat{\Sigma}_{\alpha\beta} \ll \hat{\Sigma}_{\alpha0}$, and we can neglect terms $\hat{\Sigma}_{\alpha\beta}$ with $\beta \neq 0$ and linearize the collective operator $\hat{\Sigma}_{\alpha0}$ to give

$$\hat{\Sigma}_{\alpha0} \approx \sqrt{N}\hat{a}_\alpha \quad (\alpha \neq 0). \tag{E7}$$

Substituting Eq. (E7) into Eqs. (E5-E6), we finally get

$$\hat{J}_y \approx \sqrt{2N}\sum_{\alpha=1}^4 \left(\mathrm{Re}J_{\alpha0}^y \hat{X}_\alpha + \mathrm{Im}J_{\alpha0}^y \hat{P}_\alpha\right), \tag{E8}$$

$$\hat{J}_z \approx \sqrt{2N}\sum_{\alpha=1}^4 \left(\mathrm{Re}J_{\alpha0}^z \hat{X}_\alpha + \mathrm{Im}J_{\alpha0}^z \hat{P}_\alpha\right). \tag{E9}$$

As expected, we need at most four atomic oscillators to describe the atomic system with $F=2$. Each oscillator $\hat{a}_\alpha$ is assigned to the pair of sublevels $\{\widetilde{\psi}_0^{(i)}, \widetilde{\psi}_\alpha^{(i)}\}$ with the vacuum state corresponding to no atom in the ensemble being excited from $|\widetilde{\psi}_0^{(i)}\rangle$ to $|\widetilde{\psi}_\alpha^{(i)}\rangle$, and the $n$-Fock state representing the state where $n$ atoms are transferred from $|\widetilde{\psi}_0^{(i)}\rangle$ to $|\widetilde{\psi}_\alpha^{(i)}\rangle$. The collective quadratures satisfy $(\Delta\hat{X}_\alpha)^2 = (\Delta\hat{P}_\alpha)^2 = \frac{1}{2}$ for the vacuum state. Correspondingly, under the multilevel HPA, the internal state squeezing is embodied in the matrix elements $J_{\alpha 0}^{y,z}$, which are, in turn, governed by the reference state $|\mathrm{ref}\rangle$. For the reference state $|\mathrm{CSS}\rangle$, the only nonvanishing transition matrix element are $\mathrm{Re}J_{10}^{y}$ and $\mathrm{Im}J_{10}^{z}$, leading to Eqs. (E2), while, for the reference state defined in Eq. (E3a), the nonvanishing elements would be $\mathrm{Re}J_{30}^{y}$ and $\mathrm{Im}J_{40}^{z}$, resulting in Eqs. (E4). If the reference state is a general spin squeezed state, the internal squeezing appears in a linear combination of the quadratures of the four collective oscillators—a Bogoliubov mode where the weight of each quadrature is determined by the matrix elements $J_{\alpha 0}^{y,z}$. This description will be needed to account for the interplay between the internal squeezing and the collective variance of $\hat{X}_\alpha, \hat{P}_\alpha$ and covariances of $\mathrm{Cov}(\hat{\vartheta}_\alpha, \hat{\vartheta}_\beta)$ with $\hat{\vartheta} = \hat{X}, \hat{P}$.

### 1.2 The basic theory of light-atom interaction

In our system, the probe light propagates along the $z$-axis and is linearly polarized in the $y$-direction. It interacts with the $^{87}$Rb atomic ensemble in a vapor cell at 53.5 °C. The central frequency of the probe light is blue-detuned by $\Delta$ from the D2 transition between the ground-state hyperfine level $5S_{1/2}, F=2$ and the excited-state hyperfine level $5P_{3/2}, F^{'}=3$ of the $^{87}$Rb atom. Under the condition of large detuning $\Delta$, we can apply the adiabatic elimination technique to eliminate the excited states and get the following effective Hamiltonian of light-atom interaction [S6]

$$\hat{H}_{\mathrm{int}}^{\mathrm{eff}} = -\frac{\hbar c\Gamma}{8A\Delta}\frac{\lambda^2}{2\pi}\sum_{i=1}^{N}\left\{a_1\hat{S}_z(0)\hat{F}_z^{(i)} + a_2\left[-2\hat{\Phi}\hat{F}_z^{(i)2} + 6\hat{S}_y(0)\hat{F}_y^{(i)}\right]\right\}, \tag{E10}$$

where $\hbar$ is the reduced Planck constant, c is the speed of light, and in the following text, we will take $\hbar=1, c=1$. $\Gamma = 2\pi\times 6.07$ MHz is the natural line width (FWHM) of the excited states, $\lambda = 780$ nm is wavelength of light, and $A = 7$ mm $\times$ 7 mm is the cross-section area of the light beam. $\hat{\Phi}$ is the photon flux, and $\hat{S}_{y,z}$ are optical Stokes operators of light polarization, defined by

$$\hat{\Phi} = \hat{b}_x^\dagger\hat{b}_x + \hat{b}_y^\dagger\hat{b}_y, \tag{E11a}$$
$$\hat{S}_x = \frac{1}{2}\left(\hat{b}_x^\dagger\hat{b}_x - \hat{b}_y^\dagger\hat{b}_y\right), \tag{E11b}$$
$$\hat{S}_y = \frac{1}{2}\left(\hat{b}_x^\dagger\hat{b}_y + \hat{b}_y^\dagger\hat{b}_x\right), \tag{E11c}$$
$$\hat{S}_z = \frac{1}{2i}\left(\hat{b}_x^\dagger\hat{b}_y - \hat{b}_y^\dagger\hat{b}_x\right), \tag{E11d}$$

where $\hat{b}_x(\hat{b}_y)$ and $\hat{b}_x^\dagger(\hat{b}_y^\dagger)$ are the annihilation and creation operator for the $x(y)$ polarized photons, respectively, obeying the standard commutation relation $[\hat{b}_i(z), \hat{b}_j^\dagger(z')] = \delta_{ij}\delta(z-z')$. The Stokes operators obey the commutation relations $\left[\hat{S}_y, \hat{S}_z\right] = i\hat{S}_x$. In the case of strong $x$- or $y$-linearly-polarized light, the operators $\hat{\Phi}$ and $\hat{S}_x$ can be treated as $c$-numbers, that is, $\hat{\Phi}\to\Phi$ and $\hat{S}_x \to S_x$.

For the D2 transition of $^{87}$Rb atoms starting from the hyperfine ground state $F=2$, the vector coefficient $a_1$ and the second-order tensor coefficient $a_2$ are

$$a_1 = \frac{\sqrt{2}}{100}\left(-\frac{15}{1-\Delta_{13}/\Delta} - \frac{25}{1-\Delta_{23}/\Delta} + 140\right), \tag{E12a}$$
$$a_2 = \frac{\sqrt{2}}{40}\left(\frac{1}{1-\Delta_{13}/\Delta} - \frac{5}{1-\Delta_{23}/\Delta} + 4\right). \tag{E12b}$$

where $\Delta_{13} = 2\pi\times 423.60$ MHz ($\Delta_{23} = 2\pi\times 266.65$ MHz) is the hyperfine splitting between the excited states $5P_{3/2}, F^{'}=1$ ($5P_{3/2}, F^{'}=2$) and $5P_{3/2}, F^{'}=3$. The ratio $|a_2/a_1|$ decreases as $|\Delta|$ increases. In the case of large detuning, leading to $|a_2| \ll |a_1|$, the terms proportional to $a_2$ in the Hamiltonian (E10) can be neglected, leaving only the first term known as the Faraday interaction, which can be used for QND measurements of the collective spin.

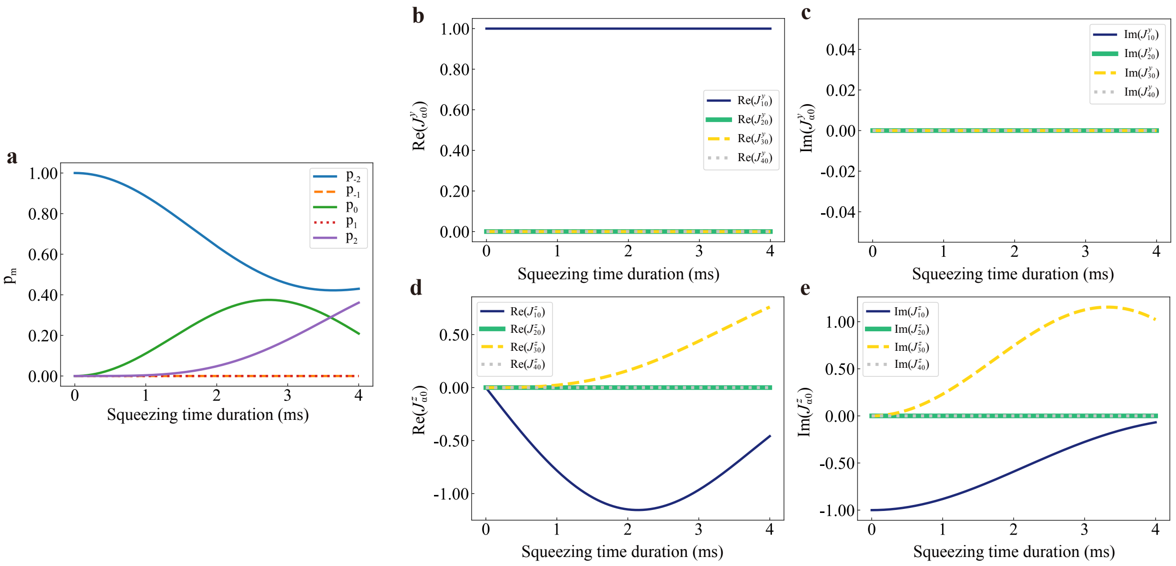


FIG. A1. (Color online) Theoretical simulation of the single-atom internal state evolution under the internal OAT interaction $\hat{H}_0^{(i)} = -\frac{1}{3}\chi_2\Phi\hat{F}_y^{(i)2}$. (a) The probability of finding a single atom in the magnetic sublevels $m_F$ versus the squeezing time. The initial state is in the $m_F = -2$ sublevel. Only the population of even-$m_F$ levels will be changed during the evolution, due to the Raman transitions between $\Delta m_F = 2$ levels. (b)-(e) The real and imaginary parts of the matrix elements $J_{\alpha 0}^k(t) = \langle\psi_\alpha^{(i)}(t)|\,\hat{F}_k^{(i)}\,|\psi_0^{(i)}(t)\rangle$ ($k = y, z$ and $\alpha = 1, 2, 3, 4$) change with the squeezing time under the interaction of $\hat{H}_0^{(i)}$. Only the matrix elements $J_{10}^z(t)$ and $J_{30}^z(t)$ change their values during the evolution, while the rest matrix elements keep unchanged.

### 1.3 The internal spin squeezing

In the language of collective spin, the interaction Hamiltonian of Eq.(E10) can be reexpressed as:

$$\hat{H} = -\frac{1}{3}\chi_2\Phi\sum_{i=1}^{N}\hat{F}_y^{(i)2} + \chi_2\hat{S}_y(0)\hat{J}_y + \chi_1\hat{S}_z(0)\hat{J}_z, \tag{E13}$$

where we have defined the new parameters $\chi_1 = -\frac{\Gamma}{8A\Delta}\frac{\lambda^2}{2\pi}a_1$ and $\chi_2 = -\frac{\Gamma}{8A\Delta}\frac{\lambda^2}{2\pi}6a_2$, corresponding to the vector and the tensor interaction strengths, respectively. The internal squeezing is created by the first OAT interaction $\hat{H}_0^{(i)} = -\frac{1}{3}\chi_2\Phi\hat{F}_y^{(i)2}$, and it leads to an evolution of a single atom from a single-atom CSS $|\psi_0^{(i)}\rangle$ to a superposition state $|\widetilde{\psi}_0^{(i)}(t)\rangle = \hat{U}_0^{(i)}(t)\,|\psi_0^{(i)}\rangle$, where $\hat{U}_0^{(i)}(t) = \mathcal{T}\,\exp\left[-i\int_0^t \hat{H}_0^{(i)}\right]$, meaning that the reference state will evolve with time. More specifically, in Fig. A1(a), we plot the probability distribution of the OAT-evolved internal state, showing that it is a supposition state with only even levels populated. Based on the physical picture outlined in Section 1.1, such a time-varying reference state will lead to changes in the atomic oscillators associated with collective spins. To clearly show the influence of internal-state evolution, we employ a rotating frame with respect to $\hat{H}_0^{(i)}$ and apply the multilevel HPA to atoms and the HPA to light, obtaining

$$\hat{H} = \kappa_2\hat{X}_1(t)\hat{x}_L(ct,t) - \kappa_1\sum_{\alpha=1}^{4}\left[\mathrm{Re}J_{\alpha 0}^z(t)\hat{X}_\alpha(t) + \mathrm{Im}J_{\alpha 0}^z(t)\hat{P}_\alpha(t)\right]\hat{p}_L(ct,t), \tag{E14}$$

where we have defined the new coupling strength $\kappa_{1,2} = \sqrt{N\Phi}\chi_{1,2}$ . The light quadrature operators $(\hat{x}_L(\xi,t), \hat{p}_L(\xi,t)) = (\hat{S}_y(ct-\xi,t), -\hat{S}_z(ct-\xi,t))/\sqrt{\Phi/2}$, where we have performed the coordinate change $\xi = ct - z$ that represents a coordinate system fixed on the optical pulse [S7]. The atomic variables are in the rotating frame: $\hat{X}_\alpha(t) = \hat{U}_0(t)\hat{X}_\alpha\hat{U}_0^\dagger(t), \hat{P}_\alpha(t) = \hat{U}_0(t)\hat{P}_\alpha\hat{U}_0^\dagger(t)$, and the time-dependent matrix elements $J_{\alpha 0}^k(t) = \langle\psi_\alpha^{(i)}(t)|\,\hat{F}_k^{(i)}\,|\psi_0^{(i)}(t)\rangle$ ($k = y, z$) are shown in Fig. A1(b-e), indicating that, for the $\hat{J}_z$ component, only the matrix elements with $\alpha = 1, 3$ are nonzero, meaning that the collective spin will be assigned with only two atomic oscillators, and, for the $\hat{J}_y$ component, only the matrix element $\mathrm{Re}J_{10}^y$ is nonzero, and is not affected by the OAT evolution as $\hat{J}_y$ commutates with $\hat{H}_0^{(i)}$.

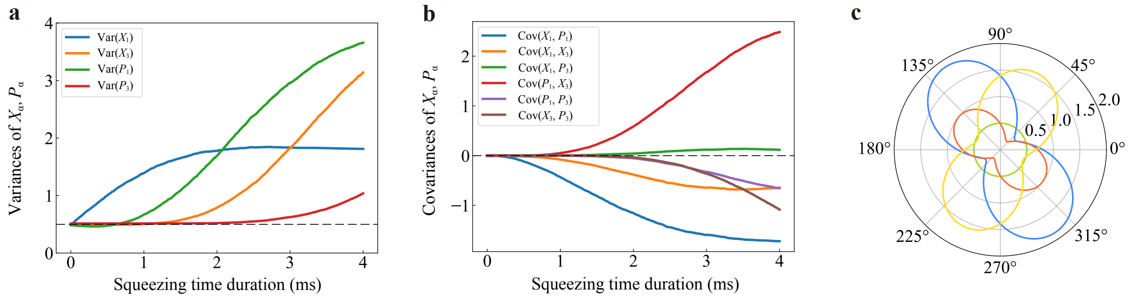


FIG. A2. (Color online) Theoretical simulation of the squeezing process induced by the Hamiltonian of Eq. (E15). (a) The variances of the collective quadratures $\hat{X}_\alpha(t)$, $\hat{P}_\alpha(t)$ ($\alpha = 1, 3$) versus squeezing time. The variance of most quadrature operators either increase or stay unchanged at the evolution time $t = 1$ ms. The black dashed line is at 0.5. (b) The covariances of the collective quadrature operators $\hat{X}_\alpha(t)$, $\hat{P}_\alpha(t)$ ($\alpha = 1, 3$) vs squeezing time duration. The black dashed line is at 0. (c) Polar plot of the normalized collective-spin variances $(\Delta \hat{J}_\theta)^2/J_x$ with $\hat{J}_\theta = \hat{J}_z \cos\theta + \hat{J}_y \sin\theta$ at the squeezing time $t = 1$ ms. The blue curve denotes the evolution results under the action of $\hat{H}$, while the red curve represents the results when only the OAT internal squeezing is present. The yellow curve shows the variances of the collective oscillator 1, obtained from the variances and covariances of quadratures $\hat{X}_1$ and $\hat{P}_1$ in (a) and (b). The green curve circle shows the variance of the CSS. The narrowest waist of each curve indicates the minimal spin variance and its direction (if any portion of the cure is within the green circle, we say that the atomic state is spin squeezed). The simulation data is estimated from 10000 Monte Carlo samples of $\hat{X}_\alpha(t)$, $\hat{P}_\alpha(t)$ whose value at time $t = 0$ is sampled from a Gaussian distribution with a mean of 0 and a variance of 0.5 and evolves over time under the action of Eq.(E15).

Consequently, the Hamiltonian (E14) is reduced to

$$\hat{H} = \kappa_2 \hat{X}_1(t)\hat{x}_L(ct,t) - \kappa_1 \sum_{\alpha=1,3} \left[ \mathrm{Re} J^z_{\alpha 0}(t)\hat{X}_\alpha(t) + \mathrm{Im} J^z_{\alpha 0}(t)\hat{P}_\alpha(t) \right] \hat{p}_L(ct,t), \tag{E15}$$

which is the Hamiltonian of Eq. (1) in the main text. Corresponding to this Hamiltonian, we evaluate the Maxwell-Bloch equations

$$\frac{d}{dt}\hat{X}_\alpha(t) = -\kappa_1 \mathrm{Im} J^z_{\alpha 0}(t)\hat{p}_L(ct,t), \tag{E16}$$

$$\frac{d}{dt}\hat{P}_\alpha(t) = -\kappa_2 \hat{x}_L(ct,t)\delta_{\alpha 1} + \kappa_1 \mathrm{Re} J^z_{\alpha 0}(t)\hat{p}_L(ct,t), \tag{E17}$$

$$\frac{\partial}{\partial t}\hat{x}_L(\xi,t) = -\kappa_1 c \sum_{\alpha=1,3} \left[ \mathrm{Re} J^z_{\alpha 0}(t)\hat{X}_\alpha(t) + \mathrm{Im} J^z_{\alpha 0}(t)\hat{P}_\alpha(t) \right] \delta(ct - \xi), \tag{E18}$$

$$\frac{\partial}{\partial t}\hat{p}_L(\xi,t) = -\kappa_2 c \hat{X}_1(t)\delta(ct - \xi). \tag{E19}$$

The equations for light can be directly integrated to give

$$\begin{aligned}\hat{x}_L(\xi,t) &= \hat{x}_L(\xi,0) - \kappa_1 c \sum_{\alpha=1,3} \int_0^t \left[ \mathrm{Re} J^z_{\alpha 0}(t)\hat{X}_\alpha(t) + \mathrm{Im} J^z_{\alpha 0}(t)\hat{P}_\alpha(t) \right] \delta(c\tau - \xi) \\ &= \hat{x}_L(\xi,0) - \kappa_1 \sum_{\alpha=1,3} \left[ \mathrm{Re} J^z_{\alpha 0}(\xi/c)\hat{X}_\alpha(\xi/c) + \mathrm{Im} J^z_{\alpha 0}(\xi/c)\hat{P}_\alpha(\xi/c) \right] \Theta\left(t - \xi/c\right),\end{aligned} \tag{E20}$$

$$\begin{aligned}\hat{p}_L(\xi,t) &= \hat{p}_L(\xi,0) - \kappa_2 c \int_0^t d\tau \hat{X}_1(\tau)\delta(c\tau - \xi) \\ &= \hat{p}_L(\xi,0) - \kappa_2 \hat{X}_1(\xi/c)\Theta\left(t - \xi/c\right),\end{aligned} \tag{E21}$$

where $\Theta(...)$ denotes the Heaviside functions. From these equations, we calculate

$$\hat{x}_L(ct,t) = \hat{x}^{\mathrm{in}}_L(t) - \frac{\kappa_1}{2} \sum_{\alpha=1,3} \left[ \mathrm{Re} J^z_{\alpha 0}(t)\hat{X}_\alpha(t) + \mathrm{Im} J^z_{\alpha 0}(t)\hat{P}_\alpha(t) \right], \tag{E22}$$

$$\hat{p}_L(ct,t) = \hat{p}^{\mathrm{in}}_L(t) - \frac{\kappa_2}{2}\hat{X}_1(t), \tag{E23}$$

where $\hat{x}_L^{\rm in}(t)=\hat{x}_L(ct,0)$ and $\hat{p}_L^{\rm in}(t)=\hat{p}_L(ct,0)$ denote the field variables before the interaction with atoms. Substituting these equations into Eqs. (E16) and (E17) yields

$$\frac{d}{dt}\hat{X}_\alpha(t) = -\kappa_1 {\rm Im}J^z_{\alpha 0}(t)\hat{p}_L^{\rm in}(t)+\frac{\kappa_1\kappa_2}{2}{\rm Im}J^z_{\alpha 0}(t)\hat{X}_1(t), \tag{E24}$$

$$\begin{aligned}\frac{d}{dt}\hat{P}_\alpha(t) &= \kappa_1 {\rm Re}J^z_{\alpha 0}(t)\hat{p}_L^{\rm in}(t)-\kappa_2\hat{x}_L^{\rm in}(t)\,\delta_{\alpha 1}\\ &+\frac{\kappa_1\kappa_2}{2}\left\{\delta_{\alpha 1}\sum_{\alpha=1,3}\left[{\rm Re}J^z_{\alpha 0}(t)\hat{X}_\alpha(t)+{\rm Im}J^z_{\alpha 0}(t)\hat{P}_\alpha(t)\right]-{\rm Re}J^z_{\alpha 0}(t)\hat{X}_1(t)\right\}.\end{aligned} \tag{E25}$$

These equations indicate that (i) due to the mediation of light, the two atomic oscillators become coupled with each other, and (ii) the evolution of the collective mode is heavily dependent on the internal state, that is, influenced by the transition matrix elements in the equations. From these equations, we are able to give the Monte Carlo simulations of the atomic oscillators evolving with time, as shown in Fig. A2.

An alternative way to calculate the variances and covariances of $\hat{X}_\alpha$, $\hat{P}_\alpha$ at any time $t$ is to derive the time-dependent covariance matrix. Forming the vector $\mathbf{x}\equiv(\hat{X}_1,\hat{P}_1,\hat{X}_3,\hat{P}_3)^T$ for atomic quadratures, we can rewrite Eqs. (E24) and (E25) as $\frac{d}{dt}\mathbf{x}(t)=\mathbf{M}(t)\mathbf{x}(t)+\mathbf{b}(t)\hat{p}_L^{\rm in}(t)+\mathbf{d}(t)\hat{x}_L^{\rm in}(t)$, where $\mathbf{M}$ is a $4\times 4$ matrix, $\mathbf{b}$ and $\mathbf{d}$ are both $4\times 1$ vectors. Introducing the covariance matrix $\mathbf{\Gamma}$ with $\Gamma_{ij}\equiv\langle(x_i-\langle x_i\rangle)(x_j-\langle x_j\rangle)\rangle$ being the element in the $i$-th row and $j$-th column, we have

$$\frac{d}{dt}\mathbf{\Gamma}(t) = \mathbf{M}(t)\mathbf{\Gamma}(t)+\mathbf{\Gamma}(t)\mathbf{M}^T(t)+\langle(\hat{p}_L^{\rm in}(t))^2\rangle\mathbf{B}(t)+\langle(\hat{x}_L^{\rm in}(t))^2\rangle\mathbf{D}(t), \tag{E26}$$

where $\mathbf{B}=\mathbf{b}\mathbf{b}^T$ and $\mathbf{D}=\mathbf{d}\mathbf{d}^T$. Using initial value of covariance matrix $\mathbf{\Gamma}(t=0)=\frac{1}{2}\mathbf{I}$, where $\mathbf{I}$ is an $4\times 4$ identity matrix, and the input light noise $\langle(\hat{p}_L^{\rm in}(t))^2\rangle=\langle(\hat{x}_L^{\rm in}(t))^2\rangle=\frac{1}{2}$, one can obtain the variances and covariances of $\hat{X}_\alpha,\hat{P}_\alpha$ at any time $t$ by numerically solving Eq. (E26).

As indicated by Eqs. (E8) and (E9), the ensemble squeezing can be achieved via either the internal squeezing (tuning the matrix elements $J^{y,z}_{\alpha 0}$) or the collective squeezing (reducing the atomic quadrature variance or creating negative covariance). To determine whether the collective modes contribute to the total squeezing, we plot in Fig. A2(a) the variance of each quadrature. The results show that almost all the variances exceed the SQL at the evolution time $t=1$ ms (corresponding to the condition of our experiment). Thus, the variances of $\hat{X}_\alpha$ or $\hat{P}_\alpha$ here will not benefit the total squeezing, but will rather reduce it. The covariance of the collective quadrature is also a key parameter in determining whether the atomic oscillator is squeezed along some other directions in phase space or whether correlations exist between different collective modes. In Fig. A2(b), we present the covariances as a function of evolution time. The results indicate that only mode 1 exhibits a significant negative covariance at the evolution time $t=1$ ms, suggesting that (i) the collective mode 1 is squeezed in some direction in phase space, and (ii) there is almost no correlation (entanglement) between the two atomic modes. As shown in Fig. A2(c), first, the squeezing of mode 1 is moderate; second, its squeezing direction substantially differs from the internal squeezing; and third, the overall squeezing direction approaches that of the internal squeezing. These results suggest that the ensemble squeezing created by the $W_1$ pulse mainly originates from the internal squeezing.

### 1.4 The collective spin squeezing

To assess the collective squeezing, a far off-resonance probe pulse $W_2$ with $y$-polarization is sent through the sample to interact with atoms through the Faraday interaction

$$\hat{H}_{\rm QND}=\chi\hat{S}_z(0)\hat{J}_z, \tag{E27}$$

where we neglected the tensorial part of the Hamiltonian (E10) as $|a_1|\gg|a_2|$ under the condition of large detuning. Because the Stokes operator $\hat{S}_z$ is a QND variable, it will not be affected by the interaction $\hat{H}_{\rm QND}$. Therefore, it is convenient to define the collective light quadratures [S2]: $\hat{X}_L=\int_0^{cT}\hat{S}_y(ct-\xi,t)d\xi/(c\sqrt{N_p/2})$, $\hat{P}_L=\int_0^{cT}\hat{S}_z(ct-\xi,t)d\xi/(c\sqrt{N_p/2})$, where $T$ is the time duration of pulse and $N_p$ is the total photon number in the pulse. The probe light is initially in the vacuum state, that is, $(\Delta X_L^{\rm in})^2=(\Delta P_L^{\rm in})^2=1/2$. Then the effective Hamiltonian turns into: $\hat{H}_{\rm QND}=\chi\sqrt{N_p/2}\hat{P}_L\hat{J}_z/T$. Corresponding to this interaction, an evaluation of the input-output relations for both

light and atoms variables yields

$$\hat{J}_y^{\text{out}} = \hat{J}_y^{\text{in}} + \chi\sqrt{N_p/2}J_x\hat{P}_L^{\text{in}}, \quad \hat{J}_z^{\text{out}} = \hat{J}_z^{\text{in}}, \tag{E28}$$

$$\hat{X}_L^{\text{out}} = \hat{X}_L^{\text{in}} - \chi\sqrt{N_p/2}\hat{J}_z^{\text{in}}, \quad \hat{P}_L^{\text{out}} = \hat{P}_L^{\text{in}}, \tag{E29}$$

where we have assumed that the atomic state after the interaction is still highly polarized along the $-x$ axis. Then, the $\hat{X}_L^{\text{out}}$ quadrature is detected via a homodyne detection. As a result, one obtains information about $\hat{J}_z$, and its variance will be reduced. To see the variance reduction, a feedback operation is performed via displacing the atomic variable $\hat{J}_z$ by an amount proportional to the measurement results, yielding the following result

$$\left(\Delta\hat{J}_z^{\text{out}}\right)^2 = \frac{1}{2}g^2 + \left(1 - g\chi\sqrt{N_p/2}\right)^2\left(\Delta\hat{J}_z^{\text{in}}\right)^2, \tag{E30}$$

where $g$ denotes the feedback gain [S8]. It can be minimized to give

$$\left(\Delta\hat{J}_z^{\text{out}}\right)^2_{\text{min}} = \frac{\left(\Delta\hat{J}_z^{\text{in}}\right)^2}{1 + \chi^2 N_p\left(\Delta\hat{J}_z^{\text{in}}\right)^2}. \tag{E31}$$

Obviously, regardless of whether the initial spin component $\hat{J}_z$ is initially squeezed or not, the QND process will further reduce its variance. It's worth noting that the pre-squeezing of $\hat{J}_z$ will decrease the efficiency of QND squeezing. This is because the atom-light coupling strength is reduced by a factor proportional to the variance of $\hat{J}_z$. From Eq. (E31), one calculates the squeezing coefficient $\xi^2 = 2(\Delta\hat{J}_z)^2/NF$ with the value

$$\xi^2 = \frac{1}{1/\xi_{\text{in}}^2 + \tilde{\kappa}^2}, \tag{E32}$$

which is the equation (2) presented in the main text. Here $\tilde{\kappa}^2 = N\Phi\chi^2 T$ denotes QND coupling strength with $T$ being the time duration of the probe pulse, and $\xi_{\text{in}}^2$ denotes the squeezing coefficient of the atomic state before the QND measurement.

To further improve the spin squeezing, we have also employed retrodiction based on later $\text{W}_2$ measurements. According to the past quantum state theory [S9, S10], if we continue measuring after $m_2$, and get the later information $m_3$ (see Fig. 1(b) in the main text), one can further reduce the variance of $m_2$, according to

$$\text{Var}(m_2|m_1, m_3) = \text{Var}(m_2) + (2I_1 - I_2 - I_3)/I_4, \tag{E33}$$

where

$$I_1 = \text{Cov}_{13}\text{Cov}_{21}Cov_{23}, \tag{E34a}$$

$$I_2 = \text{Cov}_{11}\text{Cov}_{23}^2, \tag{E34b}$$

$$I_3 = \text{Cov}_{33}\text{Cov}_{21}^2, \tag{E34c}$$

$$I_4 = \text{Cov}_{11}\text{Cov}_{33} - \text{Cov}_{13}^2. \tag{E34d}$$

with $\text{Cov}_{ij} = \text{Cov}(m_i, m_j)$ and $m_3 = \hat{S}_{y,t_3}^{\text{out}} = \int_{s_3}^{s_3+t_3}\hat{S}_y(L,t)dt$ ($s_3$ denotes the start time of the measurement of $m_3$) is the retrodiction measurement. With the help of the measurement results of $m_3$, the squeezing coefficient for this three-pulse QND scheme reads

$$\xi_{tot}^2 = \xi_{NL}^2\frac{1}{1 + (\tilde{\kappa}_1^2 + \tilde{\kappa}_3^2)\xi_{NL}^2}, \tag{E35}$$

where $\tilde{\kappa}_1 = \chi\sqrt{\Phi t_1 N}$ and $\tilde{\kappa}_3 = \chi\sqrt{\Phi t_3 N}$. Since the total pulse duration of the three-pulse scheme is approximately twice of the two-pulse scheme in experiment, it is necessary to estimate the impact of projection noise decay on the effective coupling strength during the measurement process. This can be done by appropriate modification of the term $\xi_{NL}^2 \to \frac{1}{2}(\xi_{NL}^2 + 10^{0.031})$ in the denominator of (E35), where $10^{0.031}$ denotes the experimental CSS noise with imperfection spin polarization. This modification mainly considers that the projection noise during the later retrodiction measurement of $m_3$ tends to decay more towards the noise of CSS or even thermal states, while the noise in the squeezing verification measurement of $m_2$ performed before $m_3$ undergoes less decay and is closer to the internal-SSS noise. Therefore, the effective QND coupling strength is approximated by the average of its values in internal-SSS and CSS. In Fig. 3(b) of the main text, the theoretical curve of the combined OAT and three-pulse QND squeezing is calculated by using (E35) and taking this modification into consideration.

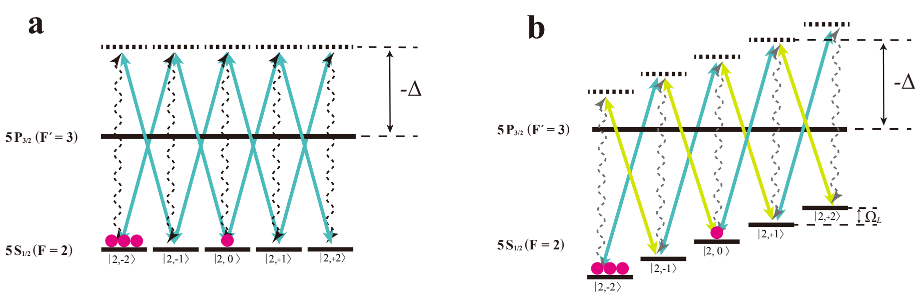


FIG. A3. (Color online) Energy levels diagrams for the interaction between the $\sigma^{\pm}$ components of the probe $W_1$ and $^{87}$Rb atom. (a) In the absence of a magnetic field, the ground states are degenerate, and the probe is not modulated (the frequency of $\sigma^+$ and $\sigma^-$ components of light is the same). (b) There is a bias magnetic field in the $x$ direction, inducing the Zeeman splitting of magnetic sublevels. The probe $W_1$ is a stroboscopic light with a square wave amplitude modulated at a frequency of twice the Larmor frequency ($2\Omega_L$). Therefore, the sidebands of the $\sigma^+$ (cyan arrow) and $\sigma^-$ (green arrow) light can interact with the two atomic sublevels $\Delta m = 2$ through two-photon resonance.

## 2. EXPERIMENTAL DETAILS

### 2.1 The stroboscopic interaction and measurement

To avoid low-frequency noise, we applied a 0.71 G bias magnetic field along the $x$ direction, which induces a Zeeman splitting with Larmor frequency of $\Omega_L \approx 2\pi \times 500$ kHz in atomic ground state. In other words, the transverse spin components $\hat{J}_y$ and $\hat{J}_z$ will rotate around the $x$ axis at the Larmor frequency $\Omega_L$.

The internal OAT spin squeezing in our experiment is generated by the Raman interaction between the equal-intensity $\sigma^{\pm}$ components of the linearly polarized probe $W_1$ and the two magnetic sublevels in the atomic ground state with $\Delta m = 2$. If there is no bias magnetic field, the ground sublevels of a single atom is degenerate, as shown in Fig. A3(a). In this case, if the frequencies of the $\sigma^+$ and $\sigma^-$ components are the same, the two-photon resonance condition can be satisfied, then the Raman interaction occurs. Conversely, if a magnetic field is applied to atoms, an energy difference $\Omega_L$ arises between two neighboring magnetic sublevels, as shown in Fig. A3(b). As a result, the two-photon detuning of $2\Omega_L$ between the $\sigma^+$ and $\sigma^-$ components of light makes the Raman process inefficient and prevents the internal spin squeezing. In the experiment, in order to eliminate the two-photon detuning, we modulated the amplitude of probe $W_1$ and turn it into a stroboscopic pulse. The modulation of the light is a square wave $\phi(t)$, which can be described by a Fourier series expansion as $\phi(t) = \sum_{k=-\infty}^{\infty} A_k e^{i2k\Omega_L t}$ with Fourier coefficients $A_k = d_1 \mathrm{sinc}(\pi k d_1)$, where $d_1 = 0.1$ is the duty cycle of the square wave on the probe $W_1$. With this setting, the probe light in frequency space is a frequency comb with a comb-tooth separation $2\Omega_L$, as shown in Fig. 1(c) in the main text. The two-photon resonance condition will be met by coupling the atoms to different sidebands of light, such as the coupling between the central-frequency and the first-sideband light.

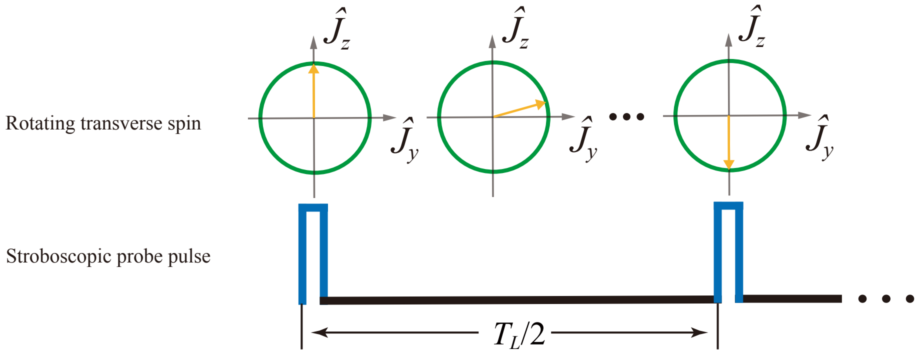


FIG. A4. (Color online) Schematics of stroboscopic measurement. We define the spin component "seen" by the first pulse (blue rectangle) of the stroboscopic probe $W_2$ as the $\hat{J}_z$ variable. Each small pulse entering the ensemble will only see $+z$ or $-z$ spin component of atoms.

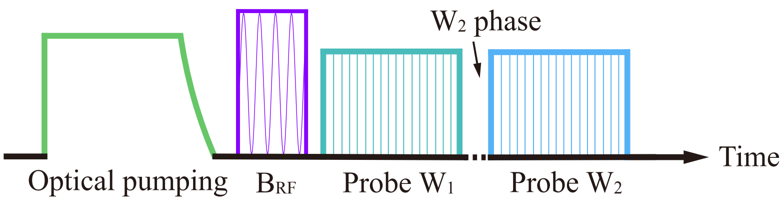


FIG. A5. (Color online) Pulse sequence of transverse mean-value measurement. $B_{RF}$ is the radio frequency magnetic field, and $W_2$ phase is the initial phase of the stroboscopic probe pulse $W_2$.

For the QND measurement, from Eq.(E28) one can see that, in the absence of magnetic field, the information about $\hat{P}_L$ will only be transferred to the $\hat{J}_y$ component of the atoms, while the $\hat{J}_z$ component remains unchanged (which is the QND variable). However, if a bias magnetic field is present in the $x$ direction, the transverse spin components $\hat{J}_y$ and $\hat{J}_z$ will rotate around the $x$ axis, then the information about $\hat{P}_L$ will be transferred to both $\hat{J}_y$ and $\hat{J}_z$, known as the back-action effect. To avoid the unwanted back-action noise induced by the magnetic field, we performed a stroboscopic measurement [S11] of $\hat{J}_z$, which is achieved by modulating probe $W_2$ into a square wave with frequency $2\Omega_L$ and duty cycle $d_2 = 0.1$, so that it could repeatedly detect the spin components $\hat{J}_z$ or $-\hat{J}_z$ for a time duration $d_2 T_L/2$ [see Fig. A4] within each half of a Larmor period.

### 2.2 Transverse mean-value measurement

In order to verify whether the OAT interaction $\hat{H}_0^{(i)}$ participates in the evolution, we perform a mean-value measurement experiment. As shown in Fig. A5, the atomic state is initially prepared in the CSS (polarized along $-x$ axis) by optical pumping. Then, a RF magnetic field $B_{RF}$ (generated by a pair of coils inside the magnetic shield) with frequency equal to Larmor frequency is applied to atoms along the $z$ axis (in laboratory frame), which creates a transverse spin mean $\langle \hat{J}_\theta \rangle \neq 0$ with $\hat{J}_\theta = \cos\theta \hat{J}_z + \sin\theta \hat{J}_y$ (in a frame rotating at the Larmor frequency). By adjusting the phase of the RF field, one can impart a mean value to an arbitrary spin component $\hat{J}_\theta$ in the $y - z$ plane. We tuned the RF phase to minimize the demodulated signal $R$ at the head of pulse $W_1$, which makes sure that, when the first time bin of $W_1$ enters the vapor cell, the non-zero mean will be created along the $y$ direction ($\langle \hat{J}_y \rangle \neq 0$) in the rotating frame. After fixing the RF phase, we first turned off the $W_1$ pulse and turned on the $W_2$ pulse to measure the collective spin. The stroboscopic measurement phase of $W_2$ (see the $W_2$ phase in Fig. A5) can be adjusted by changing the delay time of the probe pulse $W_2$. By tuning the $W_2$ phase to maximize the demodulated signal $R$ of pulse $W_2$ at $\phi_1$, the measurement direction will correspond to the mean spin direction $\hat{J}_y$. We can also measure $\hat{J}_z$ component by tuning the $W_2$ phase to $\phi_2 = \phi_1 + 90°$, and, at this moment, the corresponding observed signal $R$ will be minimal. After fixing the values of $\phi_{1,2}$, we first turned on the $W_1$ pulse to induce the $\hat{H}_0^{(i)}$ interaction, and then measured the demodulated signal $R$ of $\hat{J}_y$ and $\hat{J}_z$ components by utilizing $W_2$ at phase $\phi_1$ and $\phi_2$, respectively. Under the action of $\hat{H}_0^{(i)}$, the $\hat{J}_z$ component will have a non-zero mean value, so the direction of the mean spin in $y$-$z$ plane will no longer align with the initially direction. One can deduce the rotation angle by calculating $\arctan\langle \hat{J}_z \rangle / \langle \hat{J}_y \rangle$.

* guiyinzhang3619@zjut.edu.cn
† mfwang@wzu.edu.cn
‡ yxiao@fudan.edu.cn
[S1] T. Holstein and H. Primakoff, Phys. Rev. **58**, 1098 (1940).
[S2] Z. Kurucz and K. Mølmer, Phys. Rev. A **81**, 032314 (2010).
[S3] S. Jin, J. Duan, Y. Zhang, X. Zhang, H. Bao, H. Shen, L. Xiao, S. Jia, M. Wang, and Y. Xiao, Phys. Rev. Lett. **133**, 173604 (2024).
[S4] T. Fernholz, H. Krauter, K. Jensen, J. F. Sherson, A. S. Sørensen, and E. S. Polzik, Phys. Rev. Lett. **101**, 073601 (2008).
[S5] L. M. Norris, C. M. Trail, P. S. Jessen, and I. H. Deutsch, Phys. Rev. Lett. **109**, 173603 (2012).
[S6] B. Julsgaard, *Entanglement and quantum interactions with macroscopic gas samples*, Ph.D. thesis, University of Aarhus (2003).
[S7] C. A. Muschik, K. Hammerer, E. S. Polzik, and J. I. Cirac, Phys. Rev. A **73**, 062329 (2006).
[S8] K. Hammerer, E. S. Polzik, and J. I. Cirac, Phys. Rev. A **72**, 052313 (2005).
[S9] S. Gammelmark, B. Julsgaard, and K. Mølmer, Phys. Rev. Lett. **111**, 160401 (2013).

[S10] J. Zhang and K. Mølmer, Phys. Rev. A **96**, 062131 (2017).
[S11] H. Bao, J. Duan, S. Jin, X. Lu, P. Li, W. Qu, M. Wang, I. Novikova, E. E. Mikhailov, K.-F. Zhao, K. Mølmer, H. Shen, and Y. Xiao, Nature **581**, 159 (2020).
